# Supplementary material for: Beyond Isolation: Unlocking Reinforcement Learning Component Synergy for Sample-Efficient Continuous Control
Source: arXiv:2608.07086 source file (2026-08-07)
Supplement: Supplementary file 1 [file 0_Ethics_Statements.tex]

\clearpage
\section*{Ethics Statement}

All authors have read and adhered to the ICLR Code of Ethics.
Our research does not involve human subjects, personally identifiable information, or sensitive personal data.


\section*{Reproducibility Statement}
We provide comprehensive implementation details and experimental configurations in the appendix, including network architectures, hyperparameters, and training procedures. All experiments were conducted with multiple random seeds to ensure statistical reliability. Source code for reproducing our experimental results will be made publicly available upon acceptance.


\section*{The Use of Large Language Models}
Large language models were used during manuscript preparation for language editing, including grammar correction, sentence restructuring, and clarity improvements. 
All technical content, experimental design, analysis, and conclusions are the original work of the authors.
