# Supplementary material for: Beyond Isolation: Unlocking Reinforcement Learning Component Synergy for Sample-Efficient Continuous Control
Source: arXiv:2608.07086 source file (2026-08-07)
Supplement: Supplementary file 2 [file A_Extended_Related_Work.tex]

\newpage
\section{Related Work and Background}
\label{Related Work}
This section examines the key research areas that inform our work. We first explore 
